# Supplementary material for: DeepDPM: Deep Clustering With an Unknown Number of Clusters
Source: arXiv:2203.14309 source file (2022-03-27)
Supplement: Supplementary file 1 [file datasets.tex]

\section{Datasets}
\input{./results_files/Datasets/datasets_summary}

We evaluate and compare our approach on the following datasets, also summarized in Table~\ref{results:datasets}.
\begin{itemize}
	\item \textbf{MNIST}~\cite{Datasets:Deng:2012:MNIST}. An image dataset that has 70,000 data samples. Each sample is a 28 $\times$ 28 gray-scale image containing a handwritten digit, i.e., one of {0, 1, \dots , 9}. A number of samples from this dataset can be seen in~\autoref{datasets:mnist}.
	\input{./results_files/Datasets/MNIST_fig}
	\item \textbf{USPS~\cite{Datasets:USPS}}. An image dataset that has 9298 samples. Each sample is a 16 $\times$ 16 gray-scale image containing a handwritten digit. A few examples of this dataset can be seen in~\autoref{datasets:usps}.
	\input{./results_files/Datasets/USPS_fig}
	\item \textbf{Fashion-MNIST~\cite{Datasets:Xiao:2017:FashionMNIST}}. An MNIST-like dataset of 70,000, 28 $\times$ 28 gray-scale image labelled fashion images.
	 Some random images from this dataset can be seen in~\autoref{datasets:fashionMNIST}.
	\input{./results_files/Datasets/FashionMNIST_fig}
	\item \textbf{STL-10~\cite{Datasets:Coates:2010:STL10}}. An image dataset of 96-by-96 color images. There
are 10 classes with 1300 examples each. While it also contains 100000 unlabeled images of the same resolution, we used only the labelled samples for training for a fair comparison with the algorithms that cannot scale to the full dataset. See~\autoref{datasets:stl10} for examples.
\input{./results_files/Datasets/STL10_fig}
	\item \textbf{Reuters10k} Reuters dataset~\cite{Datasets:Lewis:2004:reuters} contains about 810000 English news stories labelled with a category tree. We followed the framework suggested by~\cite{DC:Xie:2016:DEC} and used the four root categories: corporate/industrial, government/social, markets, and economics as labels and further pruned all documents that are labelled by multiple root categories to get 685071 articles. We then computed tf-idf features on the 2000 most frequently occurring word stems. Since, unlike our method, some of the competing algorithms do not scale to the full Reuters dataset, we 
%also
sampled a random subset of 10000 examples, which we call REUTERS-10k, for comparison purposes.
\end{itemize}
