# Supplementary material for: DeepDPM: Deep Clustering With an Unknown Number of Clusters
Source: arXiv:2203.14309 source file (2022-03-27)
Supplement: Supplementary file 2 [file images_clusters.tex]

\newcommand{\myscale}{0.20}
\begin{figure}
\centering
{\includegraphics[scale=\myscale]{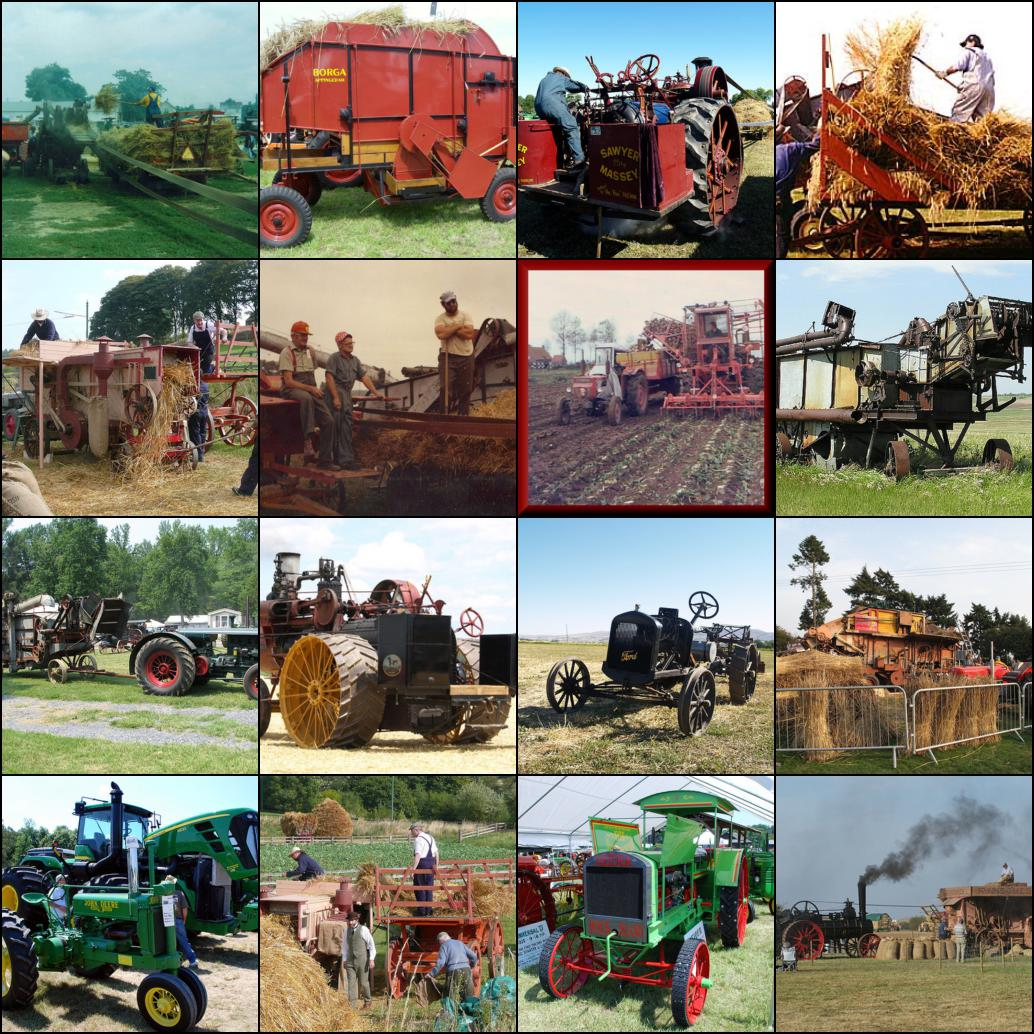}}
\caption{Examples from cluster \#1}
\label{Fig:imgs_clustered_together_sup_1}
\end{figure}

\begin{figure}
\centering
{\includegraphics[scale=\myscale]{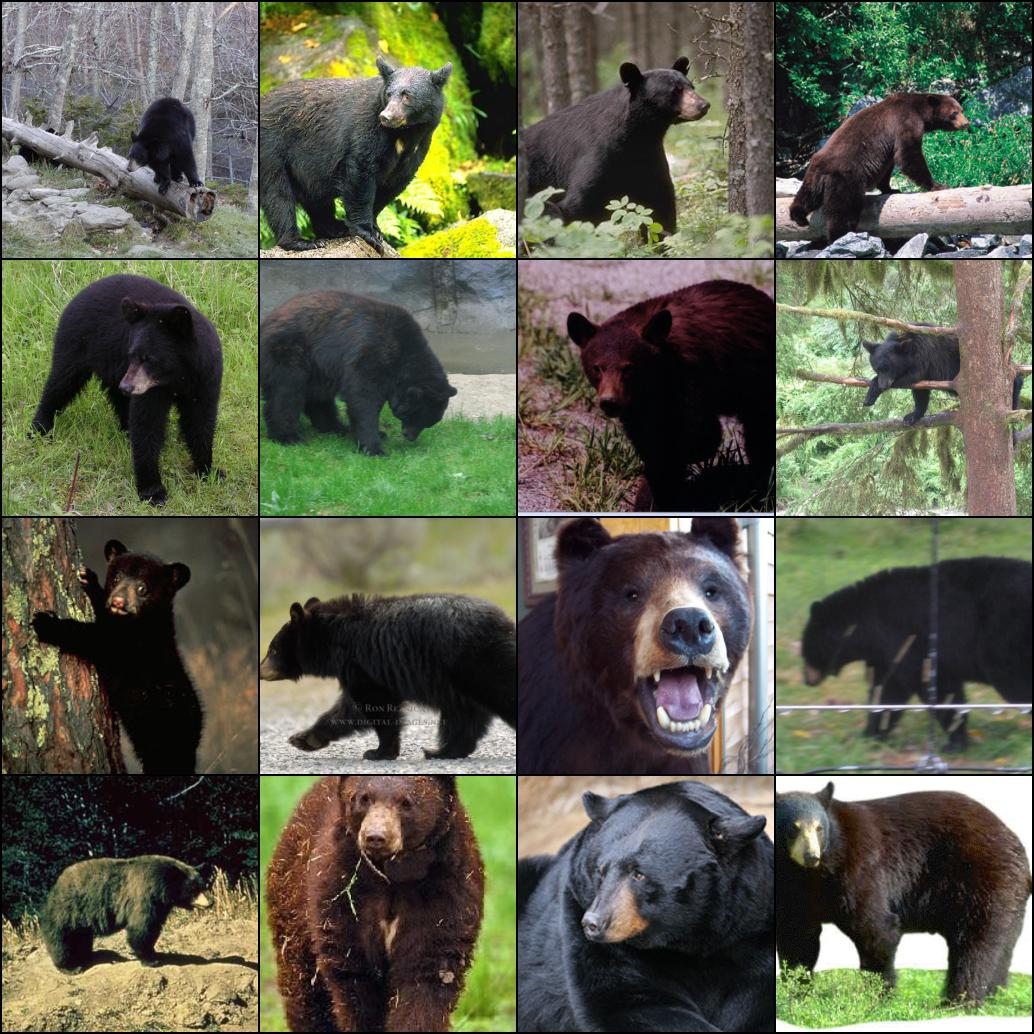}}
\caption{Examples from cluster \#2}
\label{Fig:imgs_clustered_together_sup_2}
\end{figure}

\begin{figure}
\centering
{\includegraphics[scale=\myscale]{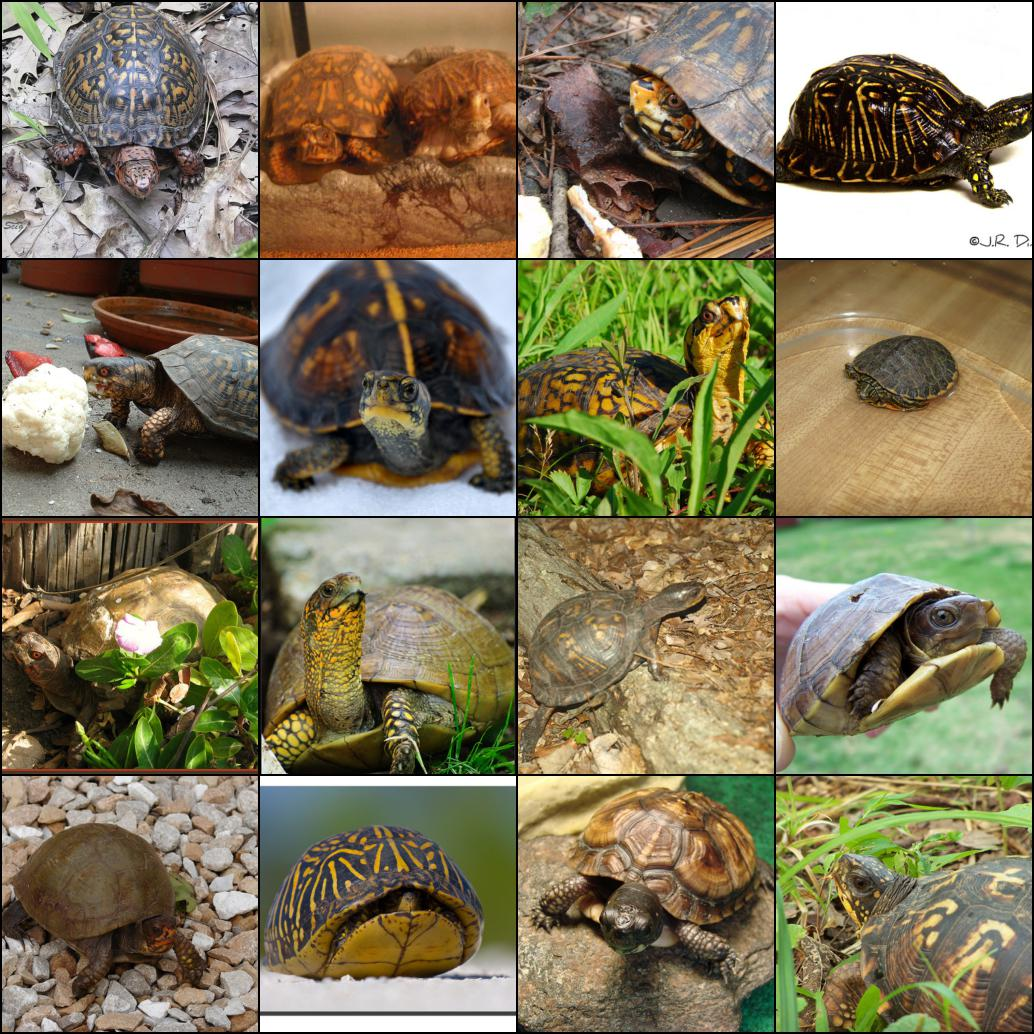}}
\caption{Examples from cluster \#3}
\label{Fig:imgs_clustered_together_sup_3}
\end{figure}

\begin{figure}
\centering
{\includegraphics[scale=\myscale]{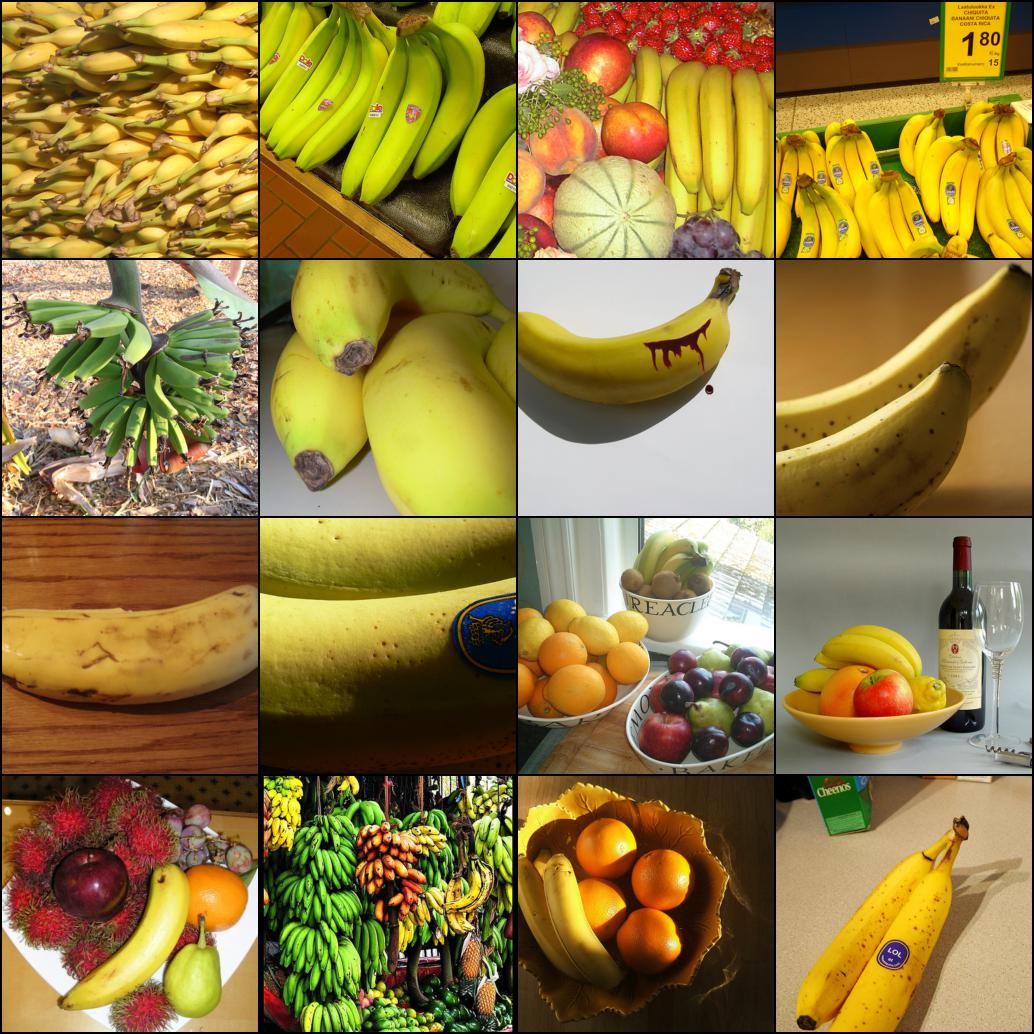}}
\caption{Examples from cluster \#4}
\label{Fig:imgs_clustered_together_sup_4}
\end{figure}

\begin{figure}
\centering
{\includegraphics[scale=\myscale]{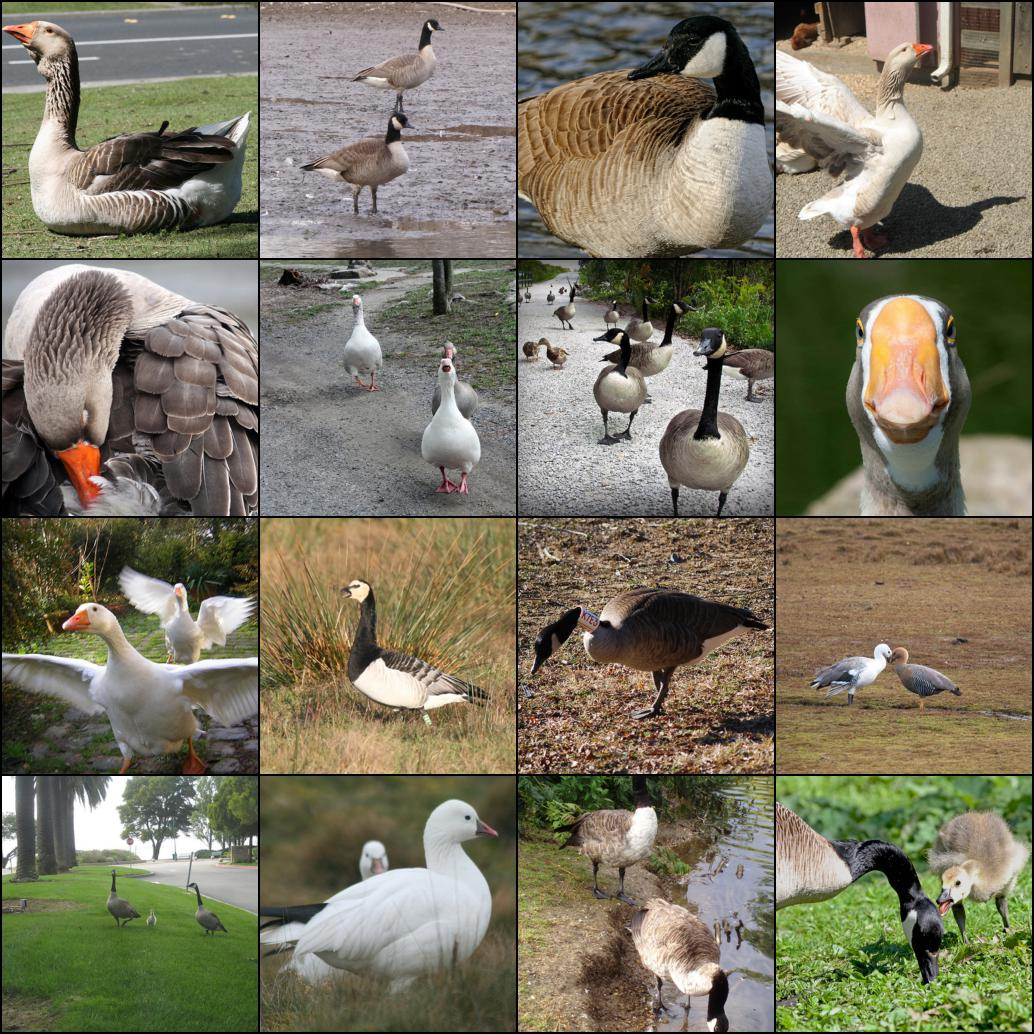}}
\caption{Examples from cluster \#5}
\label{Fig:imgs_clustered_together_sup_6}
\end{figure}

\begin{figure}
\centering
{\includegraphics[scale=\myscale]{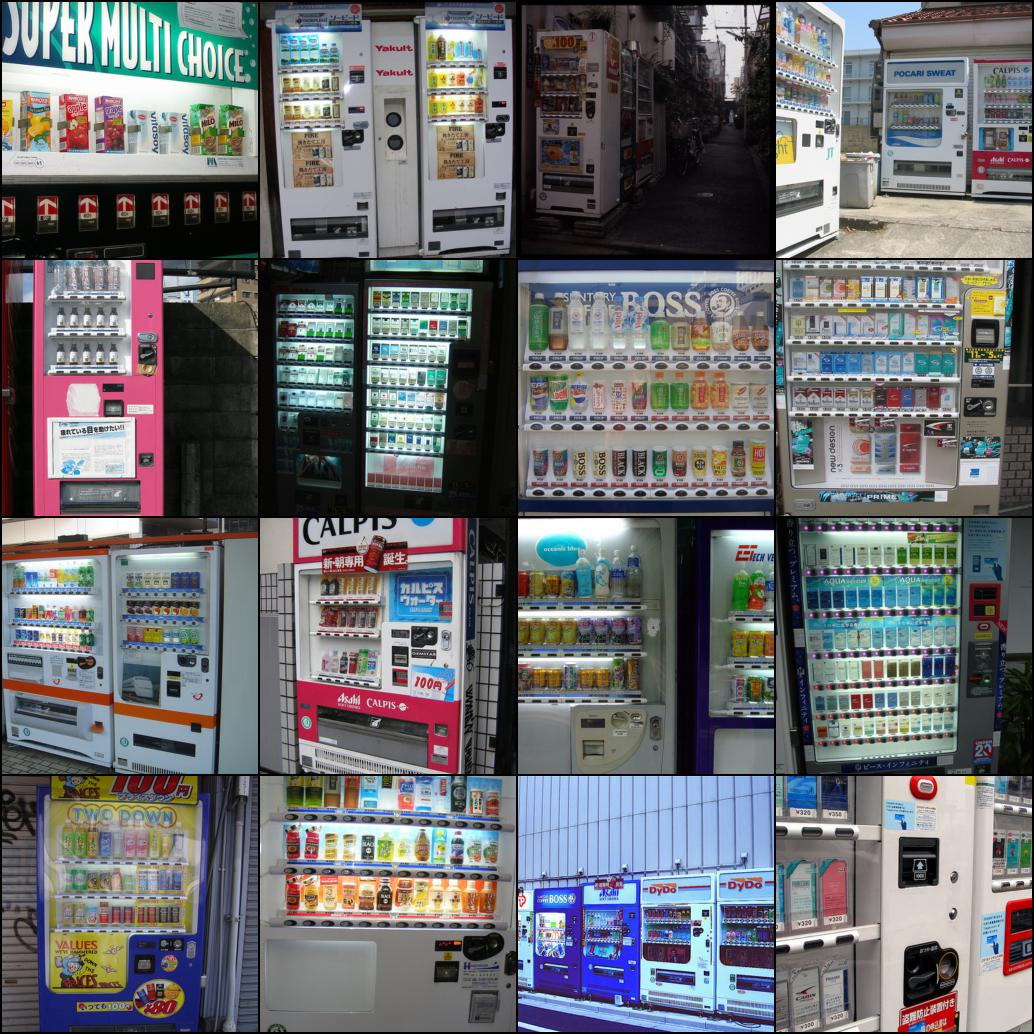}}
\caption{Examples from cluster \#6}
\label{Fig:imgs_clustered_together_sup_7}
\end{figure}

\begin{figure}
\centering
{\includegraphics[scale=\myscale]{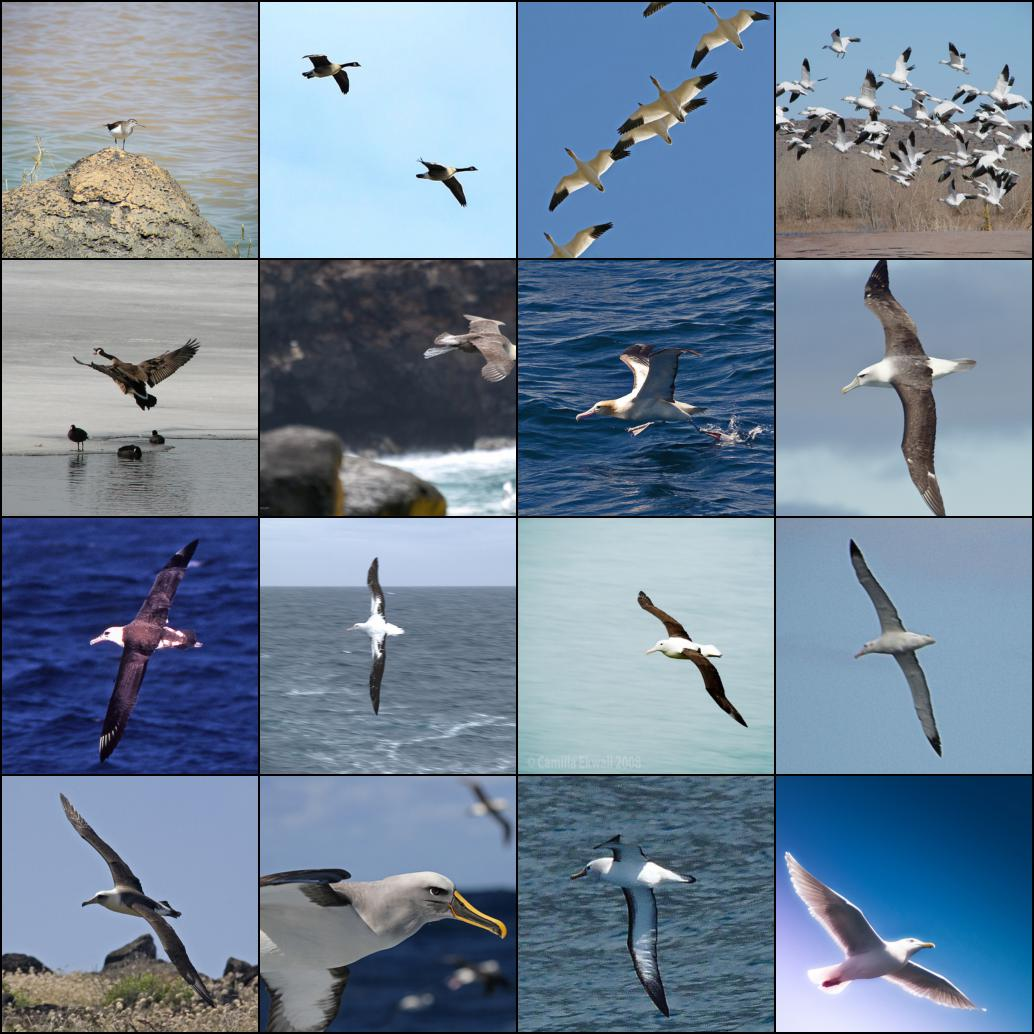}}
\caption{Examples from cluster \#7}
\label{Fig:imgs_clustered_together_sup_8}
\end{figure}

\begin{figure}
\centering
{\includegraphics[scale=\myscale]{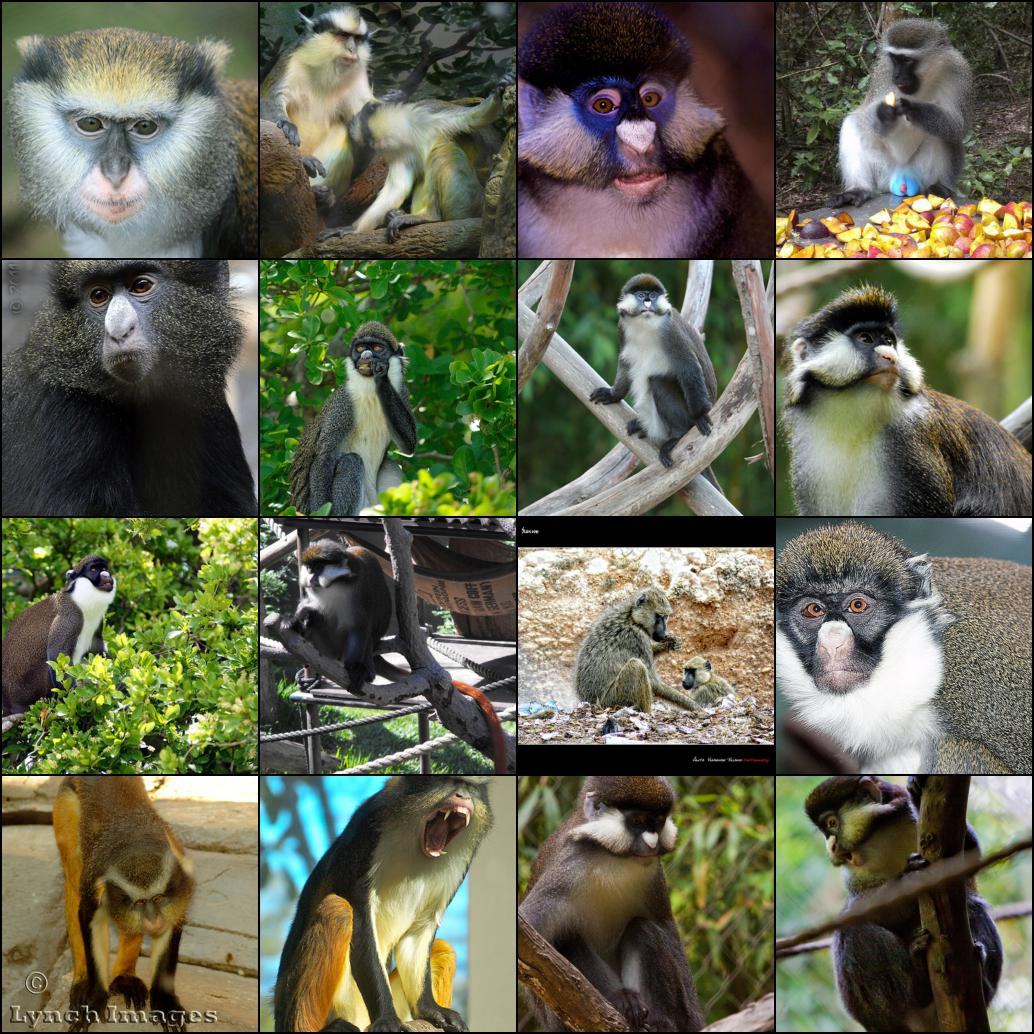}}
\caption{Examples from cluster \#8}
\label{Fig:imgs_clustered_together_sup_9}
\end{figure}
