# Supplementary material for: DeepDPM: Deep Clustering With an Unknown Number of Clusters
Source: arXiv:2203.14309 source file (2022-03-27)
Supplement: Supplementary file 5 [file final_K_imbalanced.tex]

\begin{figure}
\centerline{\includegraphics[scale=.4]{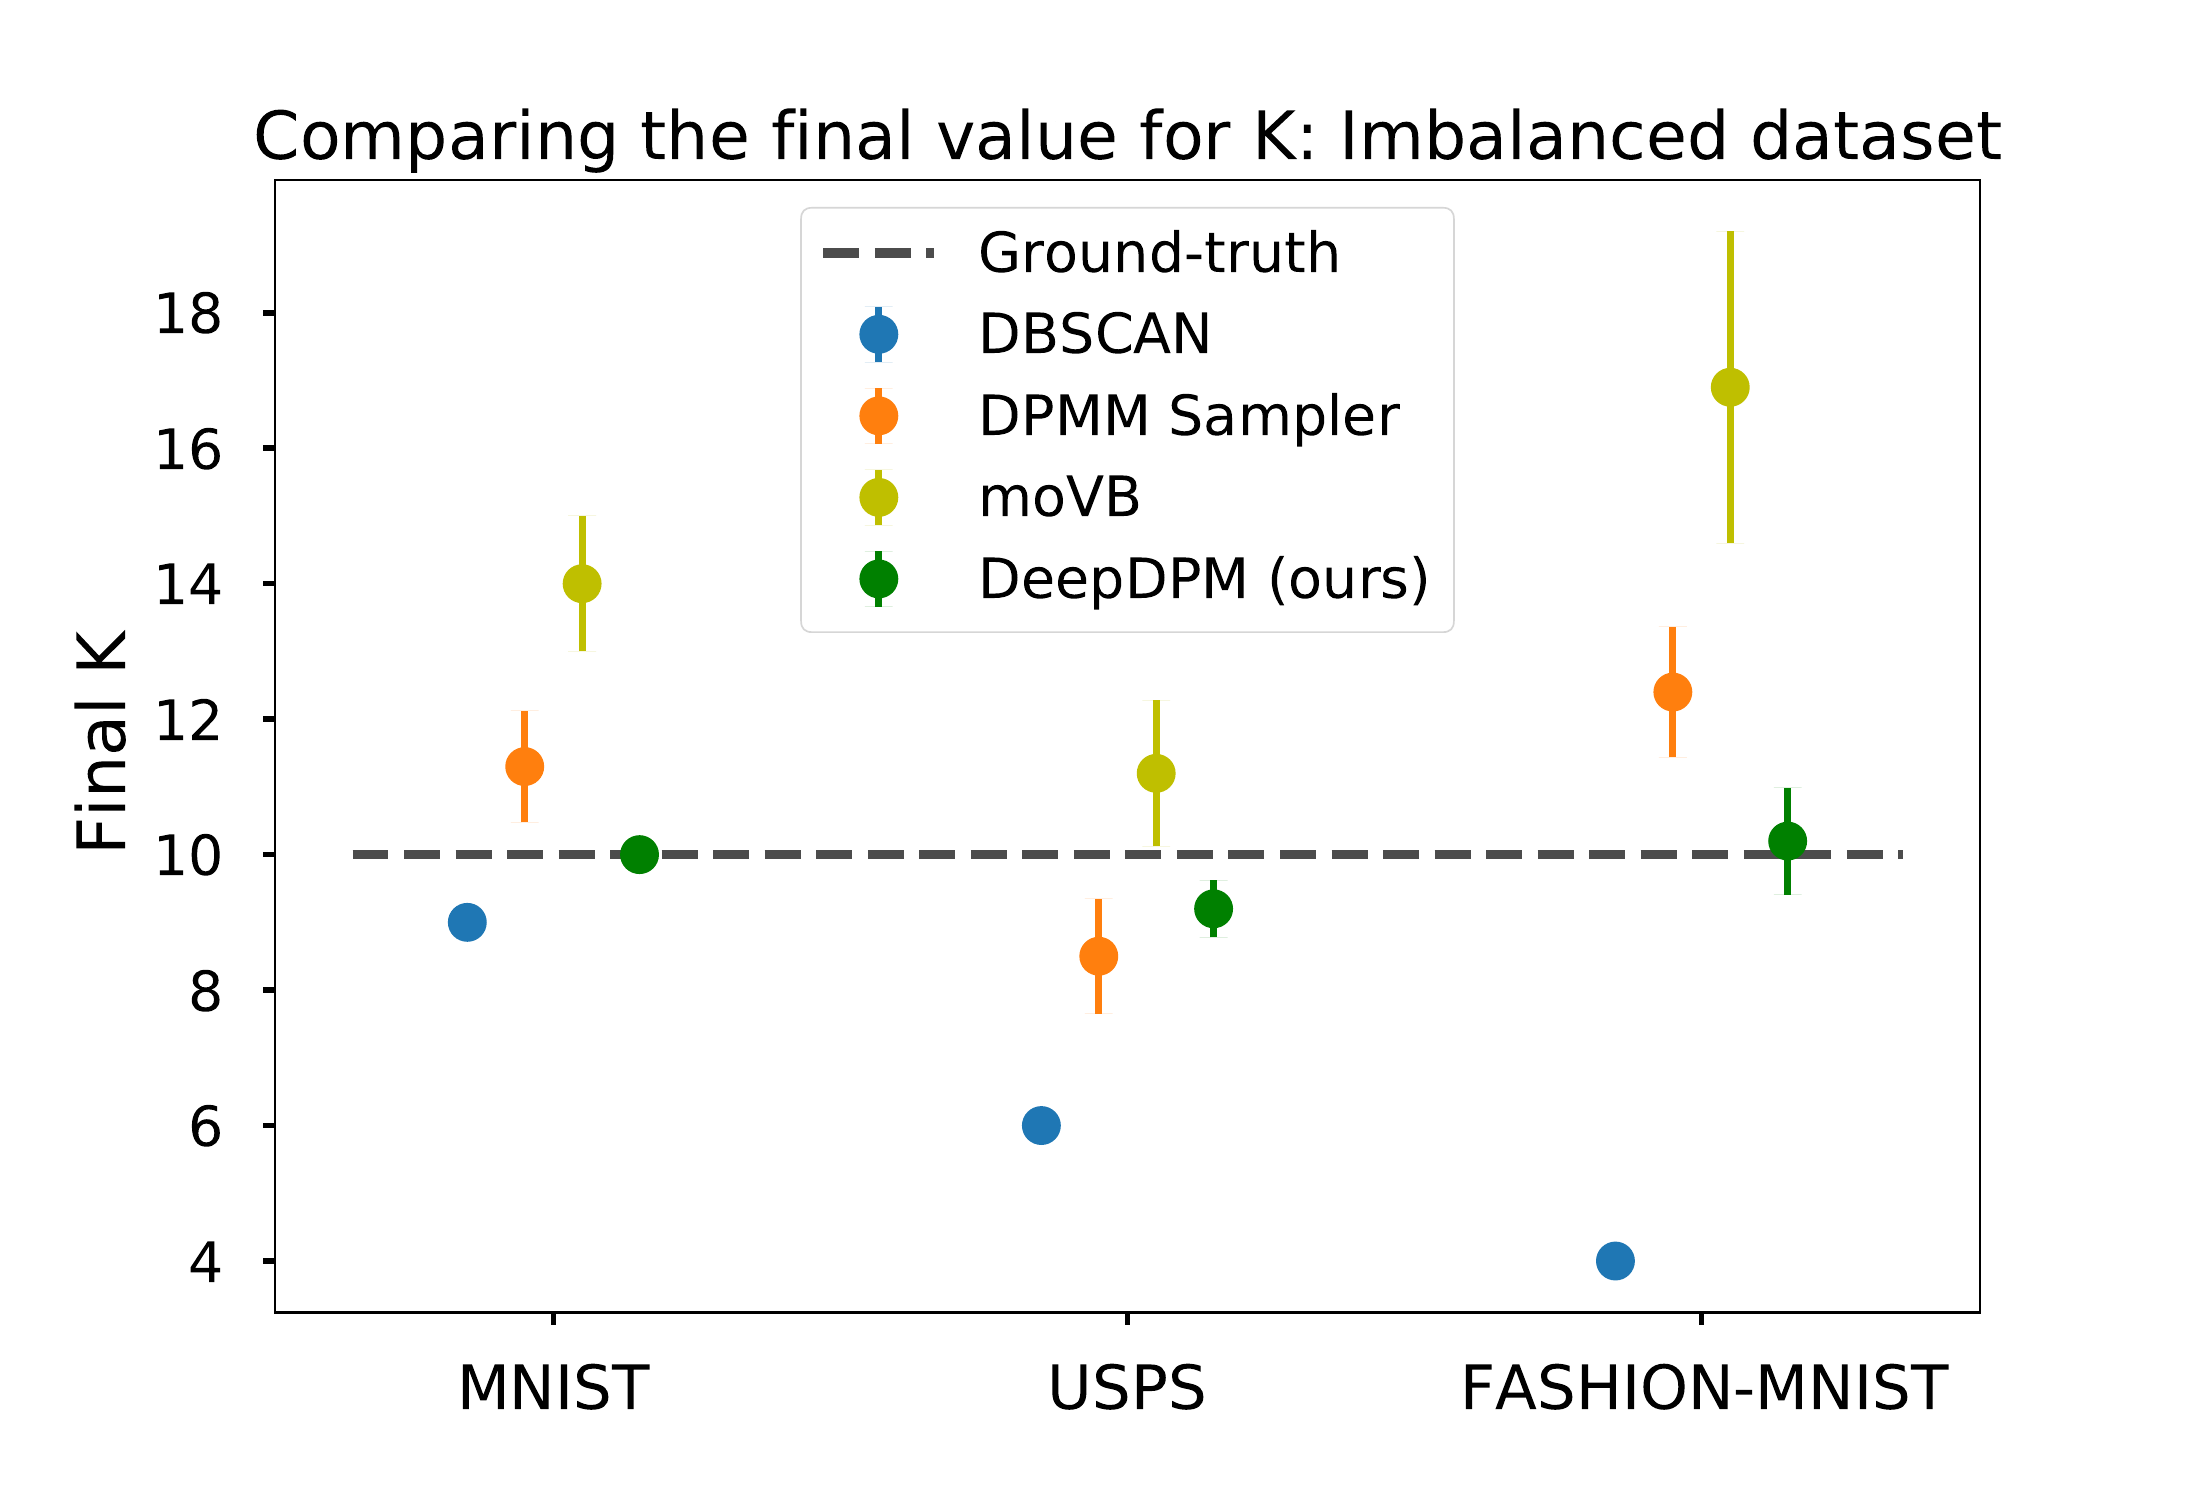}}
\caption[Comparing final K]{Comparing the inferred value of $K$ for methods which find it in imbalanced datasets. For all datasets, ground truth $K$ is 10. The dots are the mean result of 10 independent runs and the bars are the standard deviation.}
\label{results_figs:final_K_imbalanced}
\end{figure}
