# Supplementary material for: DeepDPM: Deep Clustering With an Unknown Number of Clusters
Source: arXiv:2203.14309 source file (2022-03-27)
Supplement: Supplementary file 8 [file supmat_old.tex]

% CVPR 2022 Paper Template
% based on the CVPR template provided by Ming-Ming Cheng (https://github.com/MCG-NKU/CVPR_Template)
% modified and extended by Stefan Roth (stefan.roth@NOSPAMtu-darmstadt.de)

\documentclass[10pt,twocolumn,letterpaper]{article}



\usepackage{import}
\subimport{../}{packages}
\subimport{../}{macros}

%%%%%%%%% PAPER TYPE  - PLEASE UPDATE FOR FINAL VERSION
\usepackage[review]{cvpr}      % To produce the REVIEW version
%\usepackage{cvpr}              % To produce the CAMERA-READY version
%\usepackage[pagenumbers]{cvpr} % To force page numbers, e.g. for an arXiv version

% Include other packages here, before hyperref.
\usepackage{graphicx}
\usepackage{amsmath}
\usepackage{amssymb}
\usepackage{booktabs}


% It is strongly recommended to use hyperref, especially for the review version.
% hyperref with option pagebackref eases the reviewers' job.
% Please disable hyperref *only* if you encounter grave issues, e.g. with the
% file validation for the camera-ready version.
%
% If you comment hyperref and then uncomment it, you should delete
% ReviewTempalte.aux before re-running LaTeX.
% (Or just hit 'q' on the first LaTeX run, let it finish, and you
%  should be clear).
\usepackage[pagebackref,breaklinks,colorlinks]{hyperref}


% Support for easy cross-referencing
\usepackage[capitalize]{cleveref}
\crefname{section}{Sec.}{Secs.}
\Crefname{section}{Section}{Sections}
\Crefname{table}{Table}{Tables}
\crefname{table}{Tab.}{Tabs.}


%%%%%%%%% PAPER ID  - PLEASE UPDATE
\def\cvprPaperID{4337} % *** Enter the CVPR Paper ID here
\def\confName{CVPR}
\def\confYear{2022}


% To have short pointers for sections and subsections. Oren Freifeld
\renewcommand{\sectionautorefname}{\S} 
\renewcommand{\subsectionautorefname}{\S} 
\renewcommand{\subsubsectionautorefname}{\S} 
 
\newcommand{\algorithmautorefname}{Algorithm}
\newcommand{\Exampleautorefname}{Example}


\begin{document}

%%%%%%%%% TITLE - PLEASE UPDATE
\title{%Frankly, my dear, I don't need a $K$:\\
Deep Clustering With an Unknown Number of Clusters}

\author{First Author\\
Institution1\\
Institution1 address\\
{\tt\small firstauthor@i1.org}
% For a paper whose authors are all at the same institution,
% omit the following lines up until the closing ``}''.
% Additional authors and addresses can be added with ``\and'',
% just like the second author.
% To save space, use either the email address or home page, not both
\and
Second Author\\
Institution2\\
First line of institution2 address\\
{\tt\small secondauthor@i2.org}
}

\RED{Thoughts:}
\begin{enumerate}
 \item It would be nice to mimic the table from SCAN -- (we will want ours in two versions: with pretext and with AE)           
\end{enumerate}

\RED{Vlad's Thoughts:}
\begin{enumerate}
\item What is the right $K$? (thinking about the inner-class clustering that Or has found). Maybe we should think of another metric to evaluate clustering? (an unsupervised one). Maybe add this to part in the intro where we talk about the importance of finding $K$.
\item Perform the imbalanced dataset experiments when comparing with SCAN
\item When comparing with SCAN say explicitly that they freeze their embeddings on ImageNet (to make sure the comparison is fair) and also compare on multiple datasets.
\item it is unclear what the advantages of DL are (before the sentence we say combine DL and BNP), and in general: what does our method brings compared with non-Deep ones.
\end{enumerate}

\begin{enumerate}
	\item go over the reviews of DCC to see that we don't fall in the same pitfalls: https://openreview.net/forum?id=SJzMATlAZ
	\
\end{enumerate}
Don't forget to take a look here: \url{https://github.com/otokonoko8/deep-Bayesian-nonparametrics-papers}

\subimport{./}{table_of_results.tex}


% START  (TEMP)
\pagenumbering{gobble}
\tableofcontents
\clearpage
\pagenumbering{arabic}
%  END 



\maketitle





\begin{abstract}
\subimport{./}{abstract}
\end{abstract}

\subimport{./}{intro}
\subimport{../figures/}{fig_intro}
\subimport{./}{relatedwork}
\subimport{./}{model}
\subimport{./}{method_new}
\subimport{./}{results}
\subimport{./}{conclusion}


%%%%%%%%% REFERENCES
\clearpage
{\small
\bibliographystyle{../ieee_fullname}
\bibliography{../refs}
}

\end{document}
